# Supplementary material for: Can Machines Learn Morality? The Delphi Experiment
Source: arXiv:2110.07574 source file (2022-07-12)
Supplement: Supplementary file 1 [file data_sheet.tex]

\section{Datasheet}

We include a datasheet for \dataset using the protocol defined by \cite{Gebru2021DatasheetsFD} to facilitate the reproducibility of our research.

\subsection{Motivation}

%%%%%%%%%%%%%%%%%%%%%%%%%%%%%%%%%%%%%%%%%%%%%%%%%%%%%%%%%%%%%%%%%%%%%%%%%%%%%%%%%%%%%%%%%%%%%%%%%%%%%%%%%%%%
\textbf{For what purpose was the dataset created? Was there a specific task in mind? Was there a specific gap that needed to be filled? Please provide a description.}

The Commonsense Norm Bank was created to explicitly teach large language models to be aligned with human values. We define three query-answer (QA) modes to do this:

\begin{itemize}
  \item \textbf{\Freeformmode} is the task of given a real-life situation, providing a moral judgment to the situation.
  \item \textbf{\Yesnomode} is the task of given a statement of moral judgment (\eg ``women cannot be scientists,'' ``it's kind to express concern over your neighbor's friends''), determining whether society at large would \textit{agree} or \textit{disagree} with the statement.
  \item \textbf{\Relativemode} is the task of given two situations, determining which situation has more acceptable moral implications than the other. We \textbf{exclude} this portion of the dataset from the public release of \dataset because it is not the intended use of \model. However, you can reach out to \url{delphi@allenai.org} if you would like to have access to this subsection of the dataset for research purposes.
\end{itemize}

%%%%%%%%%%%%%%%%%%%%%%%%%%%%%%%%%%%%%%%%%%%%%%%%%%%%%%%%%%%%%%%%%%%%%%%%%%%%%%%%%%%%%%%%%%%%%%%%%%%%%%%%%%%%
\textbf{Who created the dataset (\eg which team, research group) and on behalf of which entity (\eg company, institution, organization)?}

The first author created \dataset on behalf of the xlab at the Paul G. Allen School of Computer Science and the Mosaic team at the Allen Institute for Artificial Intelligence (AI2).

%%%%%%%%%%%%%%%%%%%%%%%%%%%%%%%%%%%%%%%%%%%%%%%%%%%%%%%%%%%%%%%%%%%%%%%%%%%%%%%%%%%%%%%%%%%%%%%%%%%%%%%%%%%%
\textbf{Who funded the creation of the dataset? If there is an associated grant, please provide the name of the grantor and the grant name and number.}

This dataset in itself does not require any funding as it is unified from five existing datasets: \socialchem \citep{forbes2020socialchemistry}, \ethics \citep{hendrycks2021aligning}, \moralstories \citep{emelin2020moral}, and \scruples \citep{lourie2021scruples}.
Overall, this research was funded in part by DARPA under the MCS program through NIWC Pacific (N66001-19-2-4031), and the Allen Institute for AI (AI2).

%%%%%%%%%%%%%%%%%%%%%%%%%%%%%%%%%%%%%%%%%%%%%%%%%%%%%%%%%%%%%%%%%%%%%%%%%%%%%%%%%%%%%%%%%%%%%%%%%%%%%%%%%%%%
\textbf{\textbf{Any other comments?}}

N/A

\subsection{Composition}

%%%%%%%%%%%%%%%%%%%%%%%%%%%%%%%%%%%%%%%%%%%%%%%%%%%%%%%%%%%%%%%%%%%%%%%%%%%%%%%%%%%%%%%%%%%%%%%%%%%%%%%%%%%%
\textbf{What do the instances that comprise the dataset represent (\eg documents, photos, people, countries)? Are there multiple types of instances (\eg movies, users, and ratings; people and interactions between them; nodes and edges)? Please provide a description.}

The instances from \freeformmode represents moral judgments of real-life situations, \yesnomode represents general societal agreement to moral judgments, and \relativemode represents comparison of implied moral acceptability between two situations.

%%%%%%%%%%%%%%%%%%%%%%%%%%%%%%%%%%%%%%%%%%%%%%%%%%%%%%%%%%%%%%%%%%%%%%%%%%%%%%%%%%%%%%%%%%%%%%%%%%%%%%%%%%%%
\textbf{How many instances are there in total (of each type, if appropriate)?}

There are 1.67 million instances in the \dataset in total. Here is the breakdown for the number of instances:

\begin{itemize}
  \item \Freeformmode: 1,164,810 instances
  \item \Yesnomode: 477,514 instances
  \item \Relativemode: 28,296 instances
\end{itemize}

See more detailed statistical information of \dataset broken down by source data in Table \ref{tab:unified-data-statistics}.

%%%%%%%%%%%%%%%%%%%%%%%%%%%%%%%%%%%%%%%%%%%%%%%%%%%%%%%%%%%%%%%%%%%%%%%%%%%%%%%%%%%%%%%%%%%%%%%%%%%%%%%%%%%%
\textbf{Does the dataset contain all possible instances or is it a sample (not necessarily random) of instances from a larger set? If the dataset is a sample, then what is the larger set? Is the sample representative of the larger set (\eg geographic coverage)? If so, please describe how this representativeness was validated/verified. If it is not representative of the larger set, please describe why not (\eg to cover a more diverse range of instances, because instances were withheld or unavailable).}

\textbf{What data does each instance consist of? “Raw” data (\eg unprocessed text or images) or features? In either case, please provide a description.}

\textbf{Is there a label or target associated with each instance? If so, please provide a description.}

\textbf{Is any information missing from individual instances? If so, please provide a description, explaining why this information is missing (\eg because it was unavailable). This does not include intentionally removed information, but might include, \eg redacted text.}

\textbf{Are relationships between individual instances made explicit (\eg users’ movie ratings, social network links)? If so, please describe how these relationships are made explicit.}

\textbf{Are there recommended data splits (\eg training, development/validation, testing)? If so, please provide a description of these splits, explaining the rationale behind them.}

\textbf{Are there any errors, sources of noise, or redundancies in the dataset? If so, please provide a description.}

\textbf{Is the dataset self-contained, or does it link to or otherwise rely on external resources (\eg websites, tweets, other datasets)? If it links to or relies on external resources, a) are there guarantees that they will exist, and remain constant, over time; b) are there official archival versions of the complete dataset (\ie including the external resources as they existed at the time the dataset was created); c) are there any restrictions (\eg licenses, fees) associated with any of the external resources that might apply to a dataset consumer? Please provide descriptions of all external resources and any restrictions associated with them, as well as links or other access points, as appropriate.}

\textbf{Does the dataset contain data that might be considered confidential (\eg data that is protected by legal privilege or by doctor– patient confidentiality, data that includes the content of individuals’ non-public communications)? If so, please provide a description.}

\textbf{Does the dataset contain data that, if viewed directly, might be offensive, insulting, threatening, or might otherwise cause anxiety? If so, please describe why.}

\subsection{Collection Process}

\textbf{How was the data associated with each instance acquired? Was the data directly observable (\eg raw text, movie ratings), reported by subjects (\eg survey responses), or indirectly inferred/derived from other data (\eg part-of-speech tags, model-based guesses for age or language)? If the data was reported by subjects or indirectly inferred/derived from other data, was the data validated/verified? If so, please describe how.}

\textbf{What mechanisms or procedures were used to collect the data (\eg hardware apparatuses or sensors, manual human curation, software programs, software APIs)? How were these mechanisms or procedures validated?}

\textbf{If the dataset is a sample from a larger set, what was the sampling strategy (\eg deterministic, probabilistic with specific sampling probabilities)?}

\textbf{Who was involved in the data collection process (\eg students, crowdworkers, contractors) and how were they compensated (\eg how much were crowdworkers paid)?}

\textbf{Over what timeframe was the data collected? Does this timeframe match the creation timeframe of the data associated with the instances (\eg recent crawl of old news articles)? If not, please describe the timeframe in which the data associated with the instances was created.}

\textbf{Were any ethical review processes conducted (\eg by an institutional review board)? If so, please provide a description of these review processes, including the outcomes, as well as a link or other access point to any supporting documentation.}

\subsection{Preprocessing/cleaning/labeling}

\textbf{Was any preprocessing/cleaning/labeling of the data done (\eg discretization or bucketing, tokenization, part-of-speech tagging, SIFT feature extraction, removal of instances, processing of missing values)? If so, please provide a description. If not, you may skip the remaining questions in this section.}

\textbf{Was the “raw” data saved in addition to the preprocessed/cleaned/labeled data (\eg to support unanticipated future uses)? If so, please provide a link or other access point to the “raw” data.}

\textbf{Is the software that was used to preprocess/clean/label the data available? If so, please provide a link or other access point.}

\textbf{Any other comments?}

\subsection{Uses}

\textbf{Has the dataset been used for any tasks already? If so, please provide a description.}

\textbf{Is there a repository that links to any or all papers or systems that use the dataset? If so, please provide a link or other access point.}

\textbf{What (other) tasks could the dataset be used for?}

\textbf{Is there anything about the composition of the dataset or the way it was collected and preprocessed/cleaned/labeled that might impact future uses? For example, is there anything that a dataset consumer might need to know to avoid uses that could result in unfair treatment of individuals or groups (\eg stereotyping, quality of service issues) or other risks or harms (\eg legal risks, financial harms)? If so, please provide a description. Is there anything a dataset consumer could do to mitigate these risks or harms?}

\textbf{Are there tasks for which the dataset should not be used? If so, please provide a description.}

\textbf{Any other comments?}

\subsection{Distribution}

\textbf{Will the dataset be distributed to third parties outside of the entity (\eg company, institution, organization) on behalf of which the dataset was created? If so, please provide a description.}

\textbf{How will the dataset will be distributed (\eg tarball on website, API, GitHub)? Does the dataset have a digital object identifier (DOI)?}

\textbf{When will the dataset be distributed?}

\textbf{Will the dataset be distributed under a copyright or other intellectual property (IP) license, and/or under applicable terms of use (ToU)? If so, please describe this license and/or ToU, and provide a link or other access point to, or otherwise reproduce, any relevant licensing terms or ToU, as well as any fees associated with these restrictions.}

\textbf{Have any third parties imposed IP-based or other restrictions on the data associated with the instances? If so, please describe these restrictions, and provide a link or other access point to, or otherwise reproduce, any relevant licensing terms, as well as any fees associated with these restrictions.}

\textbf{Do any export controls or other regulatory restrictions apply to the dataset or to individual instances? If so, please describe these restrictions, and provide a link or other access point to, or otherwise reproduce, any supporting documentation.}

\textbf{Any other comments?}

\subsection{Maintenance}

\textbf{Who will be supporting/hosting/maintaining the dataset?}

\textbf{How can the owner/curator/manager of the dataset be contacted (\eg email address)?}

\textbf{Is there an erratum? If so, please provide a link or other access point.}

\textbf{Will the dataset be updated (\eg to correct labeling errors, add new instances, delete instances)? If so, please describe how often, by whom, and how updates will be communicated to dataset consumers (\eg mailing list, GitHub)?}

\textbf{If the dataset relates to people, are there applicable limits on the retention of the data associated with the instances (\eg were the individuals in question told that their data would be retained for a fixed period of time and then deleted)? If so, please describe these limits and explain how they will be enforced.}

\textbf{Will older versions of the dataset continue to be supported/hosted/maintained? If so, please describe how. If not, please describe how its obsolescence will be communicated to dataset consumers}

\textbf{If others want to extend/augment/build on/contribute to the dataset, is there a mechanism for them to do so? If so, please provide a description. Will these contributions be validated/verified? If so, please describe how. If not, why not? Is there a process for communicating/distributing these contributions to dataset consumers? If so, please provide a description.}

\textbf{Any other comments?}
